# Supplementary material for: Covariance Analysis of Impulsive Streaking
Source: arXiv:2411.01729 source file (2024-12-20)
Supplement: Supplementary file 1 [file suppinfo.pdf]

Supplementary Materials for **Covariance Analysis of Impulsive Streaking**

Jun Wang *et al*

December 20, 2024

## Contents

**S1 Full Expansion of Streaking Covariance in Impulsive Regime** **1**
S1.1 Expansion up to the Fourth Order . . . . . . . . . . . . . . . . . . . . . . . . . . . . 3
S1.2 Proof of Eqn.(14) in the Main Text . . . . . . . . . . . . . . . . . . . . . . . . . . . . 4

**S2 Relation between Flux Maximization and Zero-loop Constraint** **5**

**S3 Derivation of Effects of Delay Fluctuation** **6**

**S4 Derivation of Sensitivities to Arbitrary Signals** **7**
S4.1 Reduction to Eqn.(9) When Feature Y is Impulsive . . . . . . . . . . . . . . . . . . . 10

**S5 Simulation of Auger-Meitner Feature** **11**

## S1 Full Expansion of Streaking Covariance in Impulsive Regime

The full Taylor expansion of the displacement operator is:

$$\mathcal{D}_{\boldsymbol{k}} \equiv \exp(-\boldsymbol{k}\cdot\nabla) = \sum_{l=0}^{\infty} \frac{1}{l!}(-\boldsymbol{k}\cdot\nabla)^l \; . \tag{S1}$$

The uniform distribution of $\kappa$ guarantees the expectation of any non-zeroth power of $e^{i\kappa}$ to be zero, thus it is helpful to write the dot product as a linear combination of $e^{i\kappa}$ and $e^{-i\kappa}$:

$$\boldsymbol{k}\cdot\nabla = k(\cos\kappa\partial_x + \sin\kappa\partial_y) = \frac{k}{2}\left(e^{i\kappa}(\partial_x - i\partial_y) + e^{-i\kappa}(\partial_x + i\partial_y)\right) = \frac{k}{\sqrt{2}}(e^{i\kappa}\partial_- + e^{-i\kappa}\partial_+) \; , \tag{S2}$$

where $\partial_x = \frac{\partial}{\partial x}, \partial_y = \frac{\partial}{\partial y}$ for simplicity, and $\partial_\pm \equiv (\partial_x \pm i\partial_y)/\sqrt{2}$ the same as defined in Sec. V of the main text. Substituting Eqn. (S2) into Eqn. (S1), we simplify the expectation of displacement

operator:

$$\begin{aligned}
\mathbb{E}\left[\mathcal{D}_{\boldsymbol{k}}\right] = \mathbb{E}\left[\mathbb{E}\left[\mathcal{D}_{\boldsymbol{k}}|k\right]\right] &= \mathbb{E}\left[\int_0^{2\pi}\frac{d\kappa}{2\pi}\exp\left(\frac{-k}{\sqrt{2}}\left(e^{i\kappa}\partial_- + e^{-i\kappa}\partial_+\right)\right)\right] &\text{(S3a)}\\
&= \mathbb{E}\left[\sum_{p=0}^{+\infty}\frac{1}{p!}\left(\frac{-k}{\sqrt{2}}\right)^p\int_0^{2\pi}\frac{d\kappa}{2\pi}\left(e^{i\kappa}\partial_- + e^{-i\kappa}\partial_+\right)^p\right] &\text{(S3b)}\\
&= \mathbb{E}\left[\sum_{p=0}^{+\infty}\frac{1}{p!}\left(\frac{-k}{\sqrt{2}}\right)^p\sum_{n=0}^{p}\frac{p!}{n!(p-n)!}\int_0^{2\pi}\frac{d\kappa}{2\pi}e^{i(2n-p)\kappa}\partial_-^{p-n}\partial_+^n\right] &\text{(S3c)}\\
&= \sum_{n=0}^{+\infty}\mathbb{E}\left[\left(\frac{-k}{\sqrt{2}}\right)^{2n}\frac{1}{(n!)^2}\left(\partial_-\partial_+\right)^n\right] &\text{(S3d)}\\
&= \sum_{n=0}^{+\infty}\mathbb{E}\left[\left(\frac{k}{\sqrt{2}}\right)^{2n}\right]\frac{1}{(n!)^2}\left(\frac{1}{2}\nabla^2\right)^n &\text{(S3e)}\\
&= \sum_{n=0}^{+\infty}\gamma_n(\nabla^2)^n\ , &\text{(S3f)}
\end{aligned}$$

where $\gamma_n = \langle k^{2n}\rangle/(2^{2n}(n!)^2)$ has been defined in the main text. As pointed out in the main text, the streaking vector of feature $Y$, is $\boldsymbol{k}_Y = \lambda k(\cos(\kappa+\phi)\boldsymbol{e}_x + \sin(\kappa+\phi)\boldsymbol{e}_y)$, where the factor $\lambda = \sqrt{(1+(\omega_L\tau_Y)^2)/(1+(\omega_L\tau_X)^2)}$ accounts for the possible difference from feature $X$ in streaking amplitude. This $\lambda$ factor can be absorbed into the partial derivative operators

$$\mathcal{D}_{\boldsymbol{k}_Y} = \exp(-\boldsymbol{k}_Y\cdot\nabla) = \exp\bigl(-(\lambda^{-1}\boldsymbol{k}_Y)\cdot(\lambda\nabla)\bigr)\ . \tag{S4}$$

Note that $\lambda^{-1}|\boldsymbol{k}_Y| = |\boldsymbol{k}| = k$, Eqn. (S4) indicates that the impact of this $\lambda$ factor is equivalent to scaling all first-order differentiation operators of feature $Y$ by $\lambda$ while treating the streaking amplitude as $k$.

As pointed out in the main text, the streaking covariance between two impulsive features $X$ and $Y$ is given by the operator $C[\mathcal{D}_{\boldsymbol{k}}, \mathcal{D}_{\boldsymbol{k}_Y}]$ acting on the product of dressing-free MDs:

$$\begin{aligned}
K[X,Y] &\simeq C[\mathcal{D}_{\boldsymbol{k}_X}, \mathcal{D}_{\boldsymbol{k}_Y}]\langle X^0\rangle\langle Y^0\rangle &\text{(S5a)}\\
C[\mathcal{D}_{\boldsymbol{k}_X}, \mathcal{D}_{\boldsymbol{k}_Y}] &= \mathbb{E}\left[\mathcal{D}_{\boldsymbol{k}_X}\otimes\mathcal{D}_{\boldsymbol{k}_Y}\right] - \mathbb{E}\left[\mathcal{D}_{\boldsymbol{k}_X}\right]\otimes\mathbb{E}\left[\mathcal{D}_{\boldsymbol{k}_Y}\right]\ . &\text{(S5b)}
\end{aligned}$$

Thus in addition to deriving $\mathbb{E}\left[\mathcal{D}_{\boldsymbol{k}}\right]$, we also need the expectation of operator product $\mathbb{E}\left[\mathcal{D}_{\boldsymbol{k}_X}\otimes\mathcal{D}_{\boldsymbol{k}_Y}\right]$.

Recalling that $\boldsymbol{k}_Y = \lambda k(\cos(\kappa+\phi)\boldsymbol{e}_x + \sin(\kappa+\phi)\boldsymbol{e}_y)$, we have

$$\mathbb{E}[\mathcal{D}_{\boldsymbol{k}_X} \otimes \mathcal{D}_{\boldsymbol{k}_Y}] = \mathbb{E}\left[\mathbb{E}\left[\exp\Big(-\boldsymbol{k}_X\cdot\nabla\otimes\hat{I} - \hat{I}\otimes\boldsymbol{k}_Y\cdot\nabla\Big)\Big|k\right]\right] \tag{S6a}$$

$$= \mathbb{E}\left[\int_0^{2\pi}\frac{d\kappa}{2\pi}\exp\left(\frac{-k}{\sqrt{2}}\left(e^{i\kappa}(\partial_-\otimes\hat{I} + \lambda e^{i\phi}\hat{I}\otimes\partial_-) + e^{-i\kappa}(\partial_+\otimes\hat{I} + \lambda e^{-i\phi}\hat{I}\otimes\partial_+)\right)\right)\right] \tag{S6b}$$

$$= \sum_{N=0}^{+\infty}\frac{\langle k^{2N}\rangle}{2^N(N!)^2}\Big((\partial_-\otimes\hat{I} + \lambda e^{i\phi}\hat{I}\otimes\partial_-)(\partial_+\otimes\hat{I} + \lambda e^{-i\phi}\hat{I}\otimes\partial_+)\Big)^N \tag{S6c}$$

$$= \sum_{N=0}^{+\infty}\frac{\langle k^{2N}\rangle}{2^N(N!)^2}\Big(\partial_-\partial_+\otimes\hat{I} + \lambda e^{i\phi}\partial_+\otimes\partial_- + \lambda e^{-i\phi}\partial_-\otimes\partial_+ + \lambda^2\hat{I}\otimes\partial_-\partial_+\Big)^N \tag{S6d}$$

$$= \sum_{N=0}^{+\infty}\frac{\langle k^{2N}\rangle}{2^N(N!)^2}\left(\lambda\nabla^T\otimes R(-\phi)\nabla + \frac{1}{2}(\nabla^2\otimes\hat{I} + \lambda^2\hat{I}\otimes\nabla^2)\right)^N \tag{S6e}$$

$$= \sum_{N=0}^{+\infty}\gamma_N 2^N(\hat{G}+\hat{H})^N\ , \tag{S6f}$$

where $\hat{I}$ is the identity operator, and

$$\hat{H} \equiv \frac{1}{2}\left(\nabla^2\otimes\hat{I} + \lambda^2\hat{I}\otimes\nabla^2\right) = (\partial_-\partial_+)\otimes\hat{I} + \lambda^2\hat{I}\otimes(\partial_-\partial_+) \tag{S7a}$$

$$\hat{G} \equiv \lambda\sum_{i,j}R_{ij}(-\phi)\partial_i\otimes\partial_j = \lambda e^{-i\phi}\partial_-\otimes\partial_+ + \text{c.c.} \tag{S7b}$$

have been defined in the main text, except we do not explicitly write out the $\phi$-dependence of $\hat{G}$ here, for simplicity. Hence, combining Eqn. (S6) and (S3), we obtain:

$$C[\mathcal{D}_{\boldsymbol{k}_X}, \mathcal{D}_{\boldsymbol{k}_Y}] = \mathbb{E}\left[\mathcal{D}_{\boldsymbol{k}_X}\otimes\mathcal{D}_{\boldsymbol{k}_Y}\right] - \mathbb{E}\left[\hat{\mathcal{D}}_{\boldsymbol{k}_X}\right]\otimes\mathbb{E}\left[\hat{\mathcal{D}}_{\boldsymbol{k}_Y}\right] \tag{S8a}$$

$$= \sum_{N=0}^{+\infty}2^N\gamma_N(\hat{G}+\hat{H})^N - \sum_{n=0}^{+\infty}\sum_{m=0}^{+\infty}\gamma_n\gamma_m\lambda^m(\nabla^2)^n\otimes(\nabla^2)^m\ , \tag{S8b}$$

which proved Eqn. (9) in the main text.

### S1.1 Expansion up to the Fourth Order

Up to the fourth order, equations (S3) and (S6) above are approximated as

$$\mathbb{E}\left[\mathcal{D}_{\boldsymbol{k}}\right] = 1 + \frac{\langle k^2\rangle}{4}\nabla^2 + \frac{\langle k^4\rangle}{64}(\nabla^2)^2 + o(k^5)\ , \tag{S9a}$$

$$\mathbb{E}\left[\mathcal{D}_{\boldsymbol{k}_X}\otimes\mathcal{D}_{\boldsymbol{k}_Y}\right] = 1 + \frac{\langle k^2\rangle}{2}\left(\hat{G}+\hat{H}\right) + \frac{\langle k^4\rangle}{16}\left(\hat{G}^2 + 2\hat{G}\hat{H} + \hat{H}^2\right) + o(k^5)\ . \tag{S9b}$$

Thus the operator $C[\mathcal{D}_{\boldsymbol{k}_X}, \mathcal{D}_{\boldsymbol{k}_Y}]$ is approximated as

$$\begin{aligned}
C[\mathcal{D}_{\boldsymbol{k}_X}, \mathcal{D}_{\boldsymbol{k}_Y}] =& 1 + \frac{\langle k^2\rangle}{2}(\hat{G}+\hat{H}) + \frac{\langle k^4\rangle}{16}(\hat{G}+\hat{H})^2 \\
&- \left(1 + \frac{\langle k^2\rangle}{4}\nabla^2 + \frac{\langle k^4\rangle}{64}(\nabla^2)^2\right) \otimes \left(1 + \lambda^2\frac{\langle k^2\rangle}{4}\nabla^2 + \lambda^4\frac{\langle k^4\rangle}{64}(\nabla^2)^2\right) + o(k^5) \qquad \text{(S10a)} \\
=& \frac{\langle k^2\rangle}{2}(\hat{G}+\hat{H}) + \frac{\langle k^4\rangle}{16}(\hat{G}^2 + 2\hat{G}\hat{H} + \hat{H}^2) \\
&- \left(\frac{\langle k^2\rangle}{4}(\nabla^2 \otimes I + \lambda^2 I \otimes \nabla^2) + \frac{\langle k^4\rangle}{64}(\nabla^4 \otimes I + \lambda^4 I \otimes \nabla^4) + \frac{\langle k^2\rangle^2}{16}\lambda^2\nabla^2 \otimes \nabla^2\right) + o(k^5) \\
& \qquad \text{(S10b)} \\
=& \frac{\langle k^2\rangle}{2}\hat{G} + \frac{\langle k^4\rangle}{8}\hat{G}\hat{H} + \frac{\langle k^4\rangle}{16}\hat{G}^2 + \lambda^2\frac{\langle k^4\rangle - 2\langle k^2\rangle^2}{32}\nabla^2 \otimes \nabla^2 + o(k^5) \qquad \text{(S10c)} \\
=& \underbrace{\frac{\langle k^2\rangle}{2}\hat{G}}_{(1+1)} + \underbrace{\frac{\langle k^4\rangle}{8}\hat{G}\hat{H}}_{(1+3)\&(3+1)} + \underbrace{\frac{\langle k^4\rangle}{16}\hat{R}_2 + \lambda^2\frac{\mathrm{Var}(k^2)}{16}\nabla^2 \otimes \nabla^2}_{(2+2)} + o(k^5) \qquad \text{(S10d)}
\end{aligned}$$

where $\hat{R}_2 \equiv \lambda^2 e^{-2i\phi}\partial_-^2 \otimes \partial_+^2 + c.c.$, and the corresponding $(n_X + n_Y)$ orders are labelled under each term in Eqn. (S10d). From Eqn. (S10c) to (S10d) we used the identity $\hat{R}_2 = \hat{G}^2 - \lambda^2\nabla^2 \otimes \nabla^2/2$. Note there is no $(0+2n_Y)$ or $(2n_X+0)$ orders in $C[\mathcal{D}_{\boldsymbol{k}_X}, \mathcal{D}_{\boldsymbol{k}_Y}]$, unlike in the expectation of the direct product:

$$\begin{aligned}
\mathbb{E}\left[\mathcal{D}_{\boldsymbol{k}_X} \otimes \mathcal{D}_{\boldsymbol{k}_Y}\right] &= 1 + \frac{\langle k^2\rangle}{2}(\hat{G}+\hat{H}) + \frac{\langle k^4\rangle}{16}(\hat{G}+\hat{H})^2 + o(k^5) \qquad \text{(S11a)} \\
&= 1 + \underbrace{\frac{\langle k^2\rangle}{2}\hat{G}}_{(1+1)} + \underbrace{\frac{\langle k^2\rangle}{2}\hat{H}}_{(0+2)\&(2+0)} + \underbrace{\frac{\langle k^4\rangle}{16}(\hat{R}_2 + \lambda^2\nabla^2 \otimes \nabla^2)}_{(2+2)} \\
&\quad + \underbrace{\frac{\langle k^4\rangle}{8}\hat{G}\hat{H}}_{(1+3)\&(3+1)} + \underbrace{\frac{\langle k^4\rangle}{64}(\lambda^4\hat{I} \otimes \nabla^4 + \nabla^4 \otimes \hat{I})}_{(0+4)\&(4+0)} + o(k^5)\ . \qquad \text{(S11b)}
\end{aligned}$$

## S1.2 Proof of Eqn.(14) in the Main Text

We plug in the definition of $\hat{G}$ and $\hat{H}$ into Eqn. (S10c) and then complete the square for the (1+1), (1+3) and (3+1) orders:

$$\begin{aligned}
\frac{\langle k^2\rangle}{2}\hat{G} + \frac{\langle k^4\rangle}{8}\hat{G}\hat{H} &= \frac{\langle k^2\rangle}{2}\left(\hat{G} + \underbrace{\frac{\langle k^4\rangle}{8\langle k^2\rangle}}_{\equiv a}\hat{G}\ (\nabla^2 \otimes \hat{I} + \hat{I} \otimes \lambda^2\nabla^2)\right) \qquad \text{(S12a)} \\
&= \frac{\langle k^2\rangle}{2}\sum_{i,j\in\{x,y\}} R_{ij}(-\phi)\left(\partial_i \otimes \lambda\partial_j + \partial_i(a\nabla^2) \otimes \lambda\partial_j + \partial_i \otimes \lambda^3\partial_j(a\nabla^2)\right) \qquad \text{(S12b)} \\
&= \frac{\langle k^2\rangle}{2}\sum_{i,j\in\{x,y\}} R_{ij}(-\phi)\left(\partial_i(1+a\nabla^2) \otimes \lambda\partial_j(1+a\lambda^2\nabla^2) - a^2\partial_i\nabla^2 \otimes \lambda^3\partial_j\nabla^2\right) \qquad \text{(S12c)}
\end{aligned}$$

where we have denoted $a \equiv \frac{\langle k^4 \rangle}{8\langle k^2 \rangle}$ for simplicity. The last term in Eqn. (S12c) is a (3+3) order term, so it belongs to the $o(k^5)$. Now let's substitute Eqn. (S12c) into Eqn. (S10d) and then constrain $\lambda = 1, \phi = 0$ in order to consider $K[X_q, X_{q'}]$:

$$K[X_q, X_{q'}] = \frac{\langle k^2 \rangle}{2} \sum_{i\in\{x,y\}} \tilde{\xi}_q^T \tilde{\xi}_{q'} + [(2{+}2) \text{ terms}] + o(k^5) \ , \tag{S13a}$$

$$\tilde{\xi}_q = \sqrt{\frac{\langle k^2 \rangle}{2}} \left( \nabla (1 + \frac{\langle k^4 \rangle}{8\langle k^2 \rangle} \nabla^2) \langle X^0 \rangle \right)_q \tag{S13b}$$

$$[(2{+}2) \text{ terms}] = \frac{\langle k^4 \rangle}{16} (d_q^r d_{q'}^r + d_q^i d_{q'}^i) + \frac{\mathrm{Var}(k^2)}{16} (\nabla^2 \langle X^0 \rangle)_q (\nabla^2 \langle X^0 \rangle)_{q'} \ , \tag{S13c}$$

$$d_q^r \equiv ((\partial_x^2 - \partial_y^2)\langle X^0 \rangle)_q, \quad d_q^i \equiv 2(\partial_x \partial_y \langle X^0 \rangle)_q \ , \tag{S13d}$$

where we follow the convention in the main text that subscripts $q, p$ indicates integration over the corresponding ROIs $Q_q, P_p$. We recognize that the first term in Eqn. (S13a) is the product between $\tilde{\xi}_q$ and itself, contracted over the momentum dimensions. Moreover, the sum of (2+2) terms is a matrix whose eigenvectors are all linear combinations of the second order derivatives $d^r, d^i$ and $\nabla^2 \langle X^0 \rangle$. When $\langle X^0 \rangle$ has inversion symmetry, the parity of these second order derivatives is even, as opposed to the odd parity of $\tilde{\xi}$, so the eigenvectors of the (2+2) terms are in an orthogonal subspace from $\tilde{\xi}$, which prevents the (2+2) terms from mixing with the eigenvectors of $\tilde{\xi}^T \tilde{\xi}$. As a result, the top two principal components of $\mathrm{K}_{XX}$ are in the same subspace spanned by the $x$ and $y$ components of $\tilde{\xi}$. Since $\sqrt{\frac{2}{\langle k^2 \rangle}} \tilde{\xi}$ satisfies the zero-loop constraint and approaches to $\nabla \langle X^0 \rangle$ in the small streaking amplitude regime, up to the third-order correction, the reconstructed RR gradient is

$$\xi_q = \sqrt{\frac{\langle k^2 \rangle}{2}} \int_{Q_q} d^2\boldsymbol{r} \nabla \left( 1 + \frac{\langle k^4 \rangle}{8\langle k^2 \rangle} \nabla^2 \right) \langle X^0 \rangle + o(k^4) \ . \tag{S14}$$

Similarly, for feature $Y$, the RR gradient is

$$\eta_p = \lambda \sqrt{\frac{\langle k^2 \rangle}{2}} \int_{P_p} d^2\boldsymbol{r} \nabla \left( 1 + \frac{\langle k^4 \rangle \lambda^2}{8\langle k^2 \rangle} \nabla^2 \right) \langle Y^0 \rangle + o(k^4) \ . \tag{S15}$$

## S2 Relation between Flux Maximization and Zero-loop Constraint

In Sec. III.A of the main text, we mentioned that maximizing gradient-flux $j_{\mathrm{RR}}$ necessarily satisfies the zero-loop constraint. In this supplemental section, we prove this connection between the gradient-flux $j_{\mathrm{RR}}$ and the loop-integral $l_{\mathrm{RR}}$. The gradient-flux into the loop encircled by the angular bins has been defined as

$$j_{\mathrm{RR}}(\xi) \equiv - \sum_{q=1}^{N_Q} \left( \cos\theta_q, \quad \sin\theta_q \right) \xi_q a_q \ , \tag{S16}$$

where $\xi \in \mathbb{R}_{2\times N_Q}$ is the gradient field. The loop-integral has been defined as

$$l_{\mathrm{RR}}(\xi) \equiv - \sum_{q=1}^{N_Q} \left( -\sin\theta_q, \quad \cos\theta_q \right) \xi_q a_q \ . \tag{S17}$$

In Algorithm 1 in the main text, it is specified that after obtaining the matrix $\xi^{\mathrm{P}}$ stacked by two principal components, we maximize $j_{\mathrm{RR}}(O\xi^{\mathrm{P}})$, where the variable is the 2-by-2 orthogonal matrix $O$. We parameterize the orthogonal matrix as $O = R(\chi)P$ with the rotation angle $\chi \in [0, 2\pi)$ and parity $P \in \{1, \sigma^z\}$, with $\sigma^z$ being the Pauli z matrix. Under such parameterization, the gradient-flux becomes

$$j_{\mathrm{RR}}(R(\chi)P\xi^{\mathrm{P}}) = -\sum_{q=1}^{N_Q} \begin{pmatrix}\cos\theta_q, & \sin\theta_q\end{pmatrix} R(\chi)P\xi_q^{\mathrm{P}} a_q \ . \tag{S18}$$

Meanwhile, note the property of rotation matrix $\partial R(\chi)/\partial\chi = R(\pi/2 + \chi) = R(\pi/2)R(\chi)$, the partial derivative of $j_{\mathrm{RR}}$ can be simplified as

$$\frac{\partial j_{RR}}{\partial \chi} = -\sum_{q=1}^{N_Q} \begin{pmatrix}\cos\theta_q, & \sin\theta_q\end{pmatrix} \frac{\partial R(\chi)}{\partial \chi} P\xi_q^{\mathrm{P}} a_q \tag{S19a}$$

$$= -\sum_{q=1}^{N_Q} \begin{pmatrix}\cos\theta_q, & \sin\theta_q\end{pmatrix} R(\frac{\pi}{2})R(\chi)P\xi_q^{\mathrm{P}} a_q \tag{S19b}$$

$$= \sum_{q=1}^{N_Q} \begin{pmatrix}-\sin\theta_q, & \cos\theta_q\end{pmatrix} R(\frac{\pi}{2})R(\chi)P\xi_q^{\mathrm{P}} a_q = l_{\mathrm{RR}}(R(\chi)P\xi^{\mathrm{P}}) \tag{S19c}$$

Because $\chi$ is a continuous variable, at the maximal point $\chi^*$ the partial derivative $\partial j_{\mathrm{RR}}/\partial\chi = l_{\mathrm{RR}}$ is necessarily zero, so the maximal point of the gradient flux satisfies the zero-loop condition.

## S3 Derivation of Effects of Delay Fluctuation

In Sec. IV.C of the main text, we pointed out that the impact of delay fluctuation is only ensemble averaging the covariance $C[X, Y|\phi]$ over $\phi$. Based on this observation, in this section, we derive the effect of normally distributed delay fluctuations. The probability density of the normally distributed $\phi$ follows a Gaussian function,

$$f(\phi) = \frac{1}{\sqrt{2\pi}\delta\phi} \exp\left(-\frac{(\phi - \phi_0)^2}{2\ \delta\phi^2}\right) \ , \tag{S20}$$

where $\delta\phi$ is the standard deviation (i.e. "jitter") of $\phi$, and $\phi_0$ is the mean value of $\phi$. Integrated over the normal distribution, the sinusoidal functions $\sin(m\phi), \cos(m\phi)$ are damped by the factor $\exp\left(-m^2\delta\phi^2/2\right)$:

$$\int_{-\infty}^{+\infty} d\phi \ \frac{1}{\sqrt{2\pi}\delta\phi} \exp\left(-\frac{(\phi - \phi_0)^2}{2\delta\phi^2}\right) \sin(m\phi) = \exp\left(-\frac{m^2\delta\phi^2}{2}\right) \sin(m\phi_0) \ , \tag{S21a}$$

$$\int_{-\infty}^{+\infty} d\phi \ \frac{1}{\sqrt{2\pi}\delta\phi} \exp\left(-\frac{(\phi - \phi_0)^2}{2\delta\phi^2}\right) \cos(m\phi) = \exp\left(-\frac{m^2\delta\phi^2}{2}\right) \cos(m\phi_0) \ , \tag{S21b}$$

(S21c)

In this way, the ensemble average of the GIP term is rewritten as:

$$\mathbb{E}\left[M_{\rm GIP}(\phi)\right] = \mathbb{E}\left[\frac{\langle k^2\rangle}{2}\hat{G}(\phi)\langle X^0\rangle\langle Y^0\rangle\right] = \frac{\langle k^2\rangle}{2}\mathbb{E}\left[\hat{G}(\phi)\right]\langle X^0\rangle\langle Y^0\rangle \tag{S22a}$$

$$= \frac{\langle k^2\rangle}{2}\sum_{i,j}\mathbb{E}\left[R(-\phi)\right]\partial_i\langle X^0\rangle\partial_j\langle Y^0\rangle \tag{S22b}$$

$$= \exp\left(-\frac{\delta\phi^2}{2}\right)\frac{\langle k^2\rangle}{2}\sum_{i,j}\mathbb{E}\left[R(-\phi_0)\right]\partial_i\langle X^0\rangle\partial_j\langle Y^0\rangle \tag{S22c}$$

$$= \exp\left(-\frac{\delta\phi^2}{2}\right)M_{\rm GIP}(\phi_0) \tag{S22d}$$

where in the last equation we used the fact that

$$R(-\phi) = \begin{pmatrix}\cos\phi & \sin\phi\\ -\sin\phi & \cos\phi\end{pmatrix} \tag{S23}$$

is a matrix consisting of $\cos\phi$ and $\sin\phi$.

# S4 Derivation of Sensitivities to Arbitrary Signals

This section of Supplemental text provides derivations to prove the claims in Sec. V of the main text. Applying the law of total covariance to the streaking covariance, we partitioned $K[X, Y]$ as

$$K[X,Y] = C[\mathbb{E}\left[X|\boldsymbol{k}\right], \mathbb{E}\left[Y|\boldsymbol{k}\right]] = \mathbb{E}\Big[C[\mathbb{E}\left[X|\boldsymbol{k}\right], \mathbb{E}\left[Y|\boldsymbol{k}\right]|k]\Big] + C[\mathbb{E}\left[X|k\right], \mathbb{E}\left[Y|k\right]] \ , \tag{S24}$$

where we have used $\mathbb{E}\left[\mathbb{E}\left[X|\boldsymbol{k}\right]|k\right] = \mathbb{E}\left[X|k\right]$. The reference feature $X$ is in the impulsive regime, $\mathbb{E}\left[X|\boldsymbol{k}\right] = \mathcal{D}_{\boldsymbol{k}}\langle X^0\rangle$, with such impulsive condition, Eqn. (S24) is approximated as

$$K[X,Y] \simeq \mathbb{E}\left[C[\mathcal{D}_{\boldsymbol{k}}\langle X^0\rangle, \mathbb{E}\left[Y|\boldsymbol{k}\right]|k]\right] + C[\mathbb{E}\left[\mathcal{D}_{\boldsymbol{k}}|k\right]\langle X^0\rangle, \mathbb{E}\left[Y|k\right]] \ . \tag{S25}$$

The conditional expectations inside the second term of Eqn. (S25) are

$$\mathbb{E}\left[\mathcal{D}_{\boldsymbol{k}}|k\right]\langle X^0\rangle = \sum_{b=0}^{+\infty}\frac{k^{2n}}{2^{2n}(n!)^2}(\nabla^2)^n\langle X^0\rangle \ , \tag{S26a}$$

$$\mathbb{E}\left[Y|k\right] = \int_0^{2\pi}\frac{d\kappa}{2\pi}\mathbb{E}\left[Y|\kappa,k\right] = \mathcal{Y}_0(k) \ , \tag{S26b}$$

where we follow the definition of the Fourier coefficients $\mathcal{Y}_m$ in Eqn. (19) of the main text. These coefficients depend on momentum $\boldsymbol{r}_p$, which is not written out explicitly because the following treatment applies to different individual momentum points in the same way. Recall that the confluent hypergeometric limit function is defined as

$${}_0F_1(z,x) \equiv \sum_{n=0}^{\infty}\frac{(z-1)!}{(z-1+n)!n!}x^n, \tag{S27}$$

we rewrite Eqn. (S26a) as

$$\mathbb{E}\left[\mathcal{D}_{\boldsymbol{k}}|k\right]\langle X^0\rangle = {}_0F_1\left(1, \frac{k^2\nabla^2}{4}\right)\langle X^0\rangle \equiv \mu_0(k) \ , \tag{S28}$$

where in the last equation, we invoked the definition of $\mu_0(k)$ in the main text Eqn. (21). With Equations (S26b) and (S28) substituted into Eqn. (S25), it is immediately clear that the second term is written as

$$C[\mathbb{E}\left[\mathcal{D}_{\boldsymbol{k}}|k\right]\langle X^0\rangle, \mathbb{E}\left[Y|k\right]] = C[\mu_0(k), \mathcal{Y}_0(k)] \ . \tag{S29}$$

The first term in Eqn. (S25) is the expectation of a conditional covariance, $C[\mathcal{D}_{\boldsymbol{k}}\langle X^0\rangle, \mathbb{E}\left[Y|\boldsymbol{k}\right]|k]$. Note the following identity

$$C[A,B|k] = \mathbb{E}\left[(A-\mathbb{E}\left[A|k\right])(B-\mathbb{E}\left[B|k\right])|k\right] = \int_0^{2\pi}(A-\mathbb{E}\left[A|k\right])(B-\mathbb{E}\left[B|k\right])\frac{d\kappa}{2\pi} \ , \tag{S30}$$

we substitute $A=\mathcal{D}_{\boldsymbol{k}}\langle X^0\rangle, B=\mathbb{E}\left[Y|\boldsymbol{k}\right]$ and use Eqn. (S26) to simplify this conditional covariance:

$$C[\mathcal{D}_{\boldsymbol{k}}\langle X^0\rangle, \mathbb{E}\left[Y|\boldsymbol{k}\right]|k] = \int_0^{2\pi}\left(\mathcal{D}_{\boldsymbol{k}}\langle X^0\rangle - \mathbb{E}\left[\mathcal{D}_{\boldsymbol{k}}\langle X^0\rangle|k\right]\right)\left(\mathbb{E}\left[Y|\boldsymbol{k}\right]-\mathcal{Y}_0(k)\right)\frac{d\kappa}{2\pi} \tag{S31a}$$

$$= \int \mathcal{D}_{\boldsymbol{k}}\langle X^0\rangle \ \left(\mathbb{E}\left[Y|\boldsymbol{k}\right]-\mathcal{Y}_0(k)\right)\frac{d\kappa}{2\pi} - \int \mathbb{E}\left[\mathcal{D}_{\boldsymbol{k}}\langle X^0\rangle|k\right]\left(\mathbb{E}\left[Y|\boldsymbol{k}\right]-\mathcal{Y}_0(k)\right)\frac{d\kappa}{2\pi} \tag{S31b}$$

$$= \int \mathcal{D}_{\boldsymbol{k}}\langle X^0\rangle \ \left(\mathbb{E}\left[Y|\boldsymbol{k}\right]-\mathcal{Y}_0(k)\right)\frac{d\kappa}{2\pi} - \mathbb{E}\left[\mathcal{D}_{\boldsymbol{k}}\langle X^0\rangle|k\right]\int\left(\mathbb{E}\left[Y|\boldsymbol{k}\right]-\mathcal{Y}_0(k)\right)\frac{d\kappa}{2\pi} \tag{S31c}$$

$$= \int \mathcal{D}_{\boldsymbol{k}}\langle X^0\rangle \ \left(\mathbb{E}\left[Y|\boldsymbol{k}\right]-\mathcal{Y}_0(k)\right)\frac{d\kappa}{2\pi} - \mathbb{E}\left[\mathcal{D}_{\boldsymbol{k}}\langle X^0\rangle|k\right]\left(\int \mathbb{E}\left[Y|\boldsymbol{k}\right]\frac{d\kappa}{2\pi} - \mathcal{Y}_0(k)\right) \tag{S31d}$$

$$= \int \mathcal{D}_{\boldsymbol{k}}\langle X^0\rangle \ \left(\mathbb{E}\left[Y|\boldsymbol{k}\right]-\mathcal{Y}_0(k)\right)\frac{d\kappa}{2\pi} - \mathbb{E}\left[\mathcal{D}_{\boldsymbol{k}}\langle X^0\rangle|k\right]\left(\mathcal{Y}_0(k)-\mathcal{Y}_0(k)\right) \tag{S31e}$$

$$= \int \mathcal{D}_{\boldsymbol{k}}\langle X^0\rangle \ \left(\mathbb{E}\left[Y|\boldsymbol{k}\right]-\mathcal{Y}_0(k)\right)\frac{d\kappa}{2\pi} \ . \tag{S31f}$$

Substituting Eqn. (S1) into Eqn. (S31), we further simplify this conditional covariance:

$$
\begin{aligned}
C[\mathcal{D}_{\boldsymbol{k}}\langle X^0\rangle, \mathbb{E}\left[Y|\boldsymbol{k}\right]|k] &= \int_0^{2\pi} \mathcal{D}_{\boldsymbol{k}}\langle X^0\rangle \ \left(\mathbb{E}\left[Y|\boldsymbol{k}\right] - \mathcal{Y}_0(k)\right) \frac{d\kappa}{2\pi} && \text{(S32a)}\\
&= \sum_{l=0}^{\infty} \left(\frac{-k}{\sqrt{2}}\right)^l \frac{1}{l!} \int \frac{d\kappa}{2\pi} \left(e^{i\kappa}\partial_- + e^{-i\kappa}\partial_+\right)^l \langle X^0\rangle \left(\mathbb{E}\left[Y|\boldsymbol{k}\right] - \mathcal{Y}_0(k)\right) && \text{(S32b)}\\
&= \sum_{a=0}^{\infty}\sum_{b=0}^{\infty} \left(\frac{-k}{\sqrt{2}}\right)^{a+b} \frac{1}{a!b!} \int \frac{d\kappa}{2\pi} e^{i(a-b)\kappa} \partial_-^a \partial_+^b \langle X^0\rangle \left(\mathbb{E}\left[Y|\boldsymbol{k}\right] - \mathcal{Y}_0(k)\right) && \text{(S32c)}\\
&= \sum_{a=0}^{\infty}\sum_{b=0}^{\infty} \left(\frac{-k}{\sqrt{2}}\right)^{a+b} \frac{1}{a!b!} \partial_+^b \partial_-^a \langle X^0\rangle \ \left(\mathcal{Y}_{b-a}(k) - \delta_{ab}\mathcal{Y}_0(k)\right) && \text{(S32d)}\\
&= \sum_{\substack{a,b\in\mathbb{N}\\ {\color{red}b\neq a}}} \left(\frac{-k}{\sqrt{2}}\right)^{a+b} \frac{1}{a!b!} \partial_+^n \partial_-^a \langle X^0\rangle \mathcal{Y}_{b-a}(k) && \text{(S32e)}\\
&= \left(\sum_{\substack{a,b\in\mathbb{N}\\ b>a}} + \sum_{\substack{a,b\in\mathbb{N}\\ b<a}}\right) \left(\frac{-k}{\sqrt{2}}\right)^{a+b} \frac{1}{a!b!} \partial_+^b \partial_-^a \langle X^0\rangle \mathcal{Y}_{b-a}(k) && \text{(S32f)}\\
&= \sum_{\substack{a,b\in\mathbb{N}\\ b>a}} \left(\frac{-k}{\sqrt{2}}\right)^{a+b} \frac{1}{a!b!} \partial_+^b \partial_-^a \langle X^0\rangle \ \mathcal{Y}_{b-a}(k) + \text{c.c.} && \text{(S32g)}\\
&= \sum_{m=1}^{+\infty} \left(\sum_{a=0}^{\infty} \frac{1}{a!(m+a)!} \left(\frac{-k}{\sqrt{2}}\right)^{m+2a} \partial_+^{m+a} \partial_-^a \langle X^0\rangle\right) \mathcal{Y}_m(k) + \text{c.c.} && \text{(S32h)}\\
&\equiv \sum_{m=1}^{+\infty} \mu_m(k) \mathcal{Y}_m(k) + \text{c.c.} && \text{(S32i)}
\end{aligned}
$$

From Eqn. (S32f) to Eqn. (S32g), we used the fact that $Y$ is real-valued $\mathcal{Y}_{b-a} = \mathcal{Y}^*_{a-b}$, and that $\partial_+, \partial_-$ are complex conjugate to each other. Note that $\partial_+\partial_- = \nabla^2/2$, we can simplify the factor in front of $\mathcal{Y}_m$:

$$
\begin{aligned}
\mu_m(k) &= \sum_{a=0}^{\infty} \frac{1}{a!(m+a)!} \left(\frac{-k}{\sqrt{2}}\right)^{m+2a} \partial_+^{m+a} \partial_-^a \langle X^0\rangle && \text{(S33a)}\\
&= \frac{1}{m!} \left(\frac{-k\partial_+}{\sqrt{2}}\right)^m \sum_{a=0}^{\infty} \frac{m!}{a!(m+a)!} \left(\frac{-k}{\sqrt{2}}\right)^{2a} \left(\frac{\nabla^2}{2}\right)^a \langle X^0\rangle && \text{(S33b)}\\
&= \frac{1}{m!} \left(\frac{-k\partial_+}{\sqrt{2}}\right)^m \sum_{a=0}^{\infty} \frac{m!}{(m+a)!a!} \left(\frac{k^2\nabla^2}{4}\right)^a \langle X^0\rangle && \text{(S33c)}\\
&= \frac{1}{m!} \left(\frac{-k\partial_+}{\sqrt{2}}\right)^m {}_0F_1\left(m+1, \frac{k^2\nabla^2}{4}\right) \langle X^0\rangle\ , && \text{(S33d)}
\end{aligned}
$$

where the last equation has used the definition of ${}_0F_1(z,x)$ in Eqn. (S27). We recognize that Eqn. (S33d) is identical to the sensitivity defined in Eqn. (21) in the main text. Substituting Equa-

tions (S32i) and (S29) into Eqn. (S25), we arrive at:

$$K[X,Y] \simeq \mathbb{E}\left[\sum_{s=1}^{+\infty} \mu_m(k)\mathcal{Y}_m(k) + \text{c.c.}\right] + C\left[\mu_0(k), \mathcal{Y}_0(k)\right] \tag{S34}$$

which has proved Eqn. (20) in the main text.

The encoding relation Eqn. (S34) holds for an arbitrary signal $V$ that is periodic with $\kappa$, *i.e.* the direction angle of the streaking vector of the reference feature $X$. In the example given in the main text, $V = \int_{P_p} Y(\boldsymbol{r})d\boldsymbol{r}$ is the yield of Auger-Meitner electrons in one of the momentum regions $P_p$. For another example, $V$ is the sub-cycle transient reflectivity of a piece of material driven by the dressing field, probed with the ionizing pulse in concurrence with the angular streaking measurement of $X$. Generally, the periodicity of $V$ with respect to $\kappa$ is only prerequisite for the encoding relation Eqn. (S34) to hold. With the periodicity, $V$ equals to its discrete Fourier series

$$V(\kappa, k) = \sum_{s=0}^{\infty} V_m(k) e^{is\kappa} \tag{S35a}$$

$$\mathcal{V}_m(k) = \int_0^{2\pi} V(\kappa, k) e^{-is\kappa} \frac{d\kappa}{2\pi} \ . \tag{S35b}$$

Then the streaking covariance between $X$ and $V$ is

$$K[X,V] \simeq \mathbb{E}\left[\sum_{s=1}^{+\infty} \mu_m(k)\mathcal{V}_m(k) + \text{c.c.}\right] + C\left[\mu_0(k), \mathcal{V}_0(k)\right] \tag{S36}$$

## S4.1 Reduction to Eqn.(9) When Feature Y is Impulsive

Throughout the derivations from Eqn. (S25) to Eqn. (S34), we have only made one approximation with the impulsive condition of $X \simeq \mathcal{D}_{\boldsymbol{k}} X^0$. As a result, the right hand side of Eqn. (S34) equals to the streaking covariance between the impulsive approximation $\mathcal{D}_{\boldsymbol{k}} X^0$ and feature $Y$:

$$\mathbb{E}\left[\sum_{s=1}^{+\infty} \mu_m(k)\mathcal{Y}_m(k) + \text{c.c.}\right] + C\left[\mu_0(k), \mathcal{Y}_0(k)\right] = C[\mathbb{E}\left[\mathcal{D}_{\boldsymbol{k}} X^0 | \boldsymbol{k}\right], \mathbb{E}\left[Y|\boldsymbol{k}\right]] = K[\mathcal{D}_{\boldsymbol{k}} X^0, Y] \ . \tag{S37}$$

In the cases where feature $Y$ is also in the impulsive regime, we can again approximate $Y \simeq \mathcal{D}_{\boldsymbol{k}_Y} Y^0$, which results in

$$K[\mathcal{D}_{\boldsymbol{k}} X^0, Y] \simeq K[\mathcal{D}_{\boldsymbol{k}} X^0, \mathcal{D}_{\boldsymbol{k}_Y} Y^0] = C[\mathbb{E}\left[\mathcal{D}_{\boldsymbol{k}} X^0 | \boldsymbol{k}\right], \mathbb{E}\left[\mathcal{D}_{\boldsymbol{k}_Y} Y^0 | \boldsymbol{k}\right]] \tag{S38a}$$

$$= C[\mathcal{D}_{\boldsymbol{k}}, \mathcal{D}_{\boldsymbol{k}_Y}] \langle X^0 \rangle \langle Y^0 \rangle \ . \tag{S38b}$$

Substituting Eqn. (S38b) into Eqn. (S37), the right hand side of Eqn. (S34) is written as

$$\mathbb{E}\left[\sum_{s=1}^{+\infty} \mu_m(k)\mathcal{Y}_m(k) + \text{c.c.}\right] + C\left[\mu_0(k), \mathcal{Y}_0(k)\right] \simeq C[\mathcal{D}_{\boldsymbol{k}}, \mathcal{D}_{\boldsymbol{k}_Y}] \langle X^0 \rangle \langle Y^0 \rangle \ , \tag{S39}$$

where the full-series of operator $C[\mathcal{D}_{\boldsymbol{k}}, \mathcal{D}_{\boldsymbol{k}_Y}]$ has been elaborated in Eqn. (9) in the main text. This indicates that under the impulsive approximation of $Y$, the general expression (Eqn. (20) in the main text) reduces to the result of $C[\mathcal{D}_{\boldsymbol{k}}, \mathcal{D}_{\boldsymbol{k}_Y}]$ operator acting on the product distribution $\langle X^0 \rangle \langle Y^0 \rangle$.

## S5 Simulation of Auger-Meitner Feature

In Sec. V of the main text, a simulated Auger-Meitner (AM) distribution served as an example of a non-impulsive feature. This simulation is also based on the strong-field approximation, and it follows a similar form as Eq. (1) in the main text to calculate the probability amplitude:

$$b(\boldsymbol{p},\boldsymbol{p}_p;\boldsymbol{A}) = \int_{t_0}^{\infty} dt_2 e^{-i\Phi(t_2;\boldsymbol{p},\boldsymbol{A})} \sum_{\alpha=A,B} G_\alpha(t_2,\boldsymbol{p}-e\boldsymbol{A}(t_2),\boldsymbol{p}_p) \ , \tag{S40}$$

$$G_\alpha(t_2,\boldsymbol{p}_2,\boldsymbol{p}_p) = \int_{t_0}^{t_2} dt_1 e^{i\boldsymbol{p}_p^2(t_1-t_0)/(2m\hbar)+i(I_\alpha-i\Gamma/2)(t_1-t_0)/\hbar} D(\boldsymbol{p}_p) E_X(t_1) e^{+i(I^{(2)}-I_\alpha+i\Gamma/2)(t_2-t_0)/\hbar} \ , \tag{S41}$$

where $\boldsymbol{p}_p$ is the momentum of photoelectron ionized from the core-level orbital by the x-ray pulse, $I_A = 291.30\,\mathrm{eV}, I_B = 295.99\,\mathrm{eV}$ are the ionization potential to the core-excited cationic states, $\Gamma = 1/6\,\mathrm{fs}^{-1}$ is the inverse core-vacancy lifetime, $I^{(2)} = 35.50\,\mathrm{eV}$ is the energy of a dication state that both core-excited cationic states decay into, and other symbols follow the same definitions as the main text. In this example, both the $360\,\mathrm{eV}$, $0.21\,\mathrm{fs}$ x-ray pulse $E_X(t)$ and the $1.85\,\mu\mathrm{m}, 700\,\mathrm{fs}$ are assumed to be Fourier transform-limited Gaussian pulses with maximal intensity at $t = 0$. The integral starts at $t_0 = -2.5\,\mathrm{fs}$, well before the onset of the x-ray pulse. Here $b(\boldsymbol{p},\boldsymbol{p}_p;\boldsymbol{A})$ represents the complex probability amplitude associated with a specific dicationic state in the final three-body (two electrons and one dication) system, given the vector potential of the streaking field as $\boldsymbol{A}(t)$. Without discriminating the photoelectrons, the corresponding momentum distribution of the AM electron is given by

$$Y(\boldsymbol{p};\boldsymbol{k}=e\boldsymbol{A}(0)) = \int d^3\boldsymbol{p}_p |b(\boldsymbol{p},\boldsymbol{p}_p;\boldsymbol{A})|^2 \ , \tag{S42}$$

where we have assumed the photoemission delay of the $> 60\,\mathrm{eV}$ photoelectron to be negligible, and so the streaking vector $\boldsymbol{k}$ is given by $e\boldsymbol{A}(0)$. Since for an arbitrary rotation $\hat{R}$ about the x-ray propagation direction the Volkov phase is invariant $\Phi(t;\hat{R}\boldsymbol{p},\hat{R}\boldsymbol{A}) = \Phi(t;\boldsymbol{p},\boldsymbol{A})$, and that $G_\alpha$ is angularly isotropic with $\boldsymbol{p}_2$, the probability density is invariance when the AM momentum $\boldsymbol{p}$ and the vector potential $\boldsymbol{A}(t)$ are rotated by the same $\hat{R}$, *i.e.* $Y(\hat{R}\boldsymbol{p};\hat{R}\boldsymbol{k}) = Y(\boldsymbol{p};\boldsymbol{k})$. As described in the main text, we only simulated the MD on the $p_z = 0$ plane.
